# Supplementary material for: PsycheMME: A Psychology-Informed Benchmark for Social Understanding and Interaction in Videos
Source: arXiv:2610.28625 source file (2026-10-20)
Supplement: Supplementary file 1 [file extended_methodology.tex]

% ================================================================
% PsycheMME - detailed supplementary methodology
%
% INTEGRATION:
%   After \appendix and AFTER the bibliography, insert
%       \input{sections/appendix/extended_methodology}
%   (adjust directory to your project).
%
% This file is intended to REPLACE the existing Appendix A
% ``Taxonomy Definitions and Boundaries'', not to be appended
% alongside it: the earlier A.1-A.4 content is integrated here.
% The existing Appendix B (Experimental Details) may follow.
% No figure is repeated in this appendix.
% ================================================================
\section{Extended Methodology}
\label{app:methodology}

This appendix expands the task formulation, capability definitions,
benchmark construction, and scoring protocol in
Section~\ref{sec:methodology}. It clarifies the boundaries on interpreting cues and making inferences used to design PsycheMME. Illustrative situations below
explain distinctions between capabilities; they are not additional
benchmark samples or controlled empirical comparisons.

\subsection{Theoretical Motivation and Capability Taxonomy}
\label{app:taxonomy_details}

\paragraph{Theoretical organization.}
Social Information Processing (SIP) distinguishes the encoding and
interpretation of social cues from goal clarification and response
selection~\cite{crick1994sip}. The Perception-Action Cycle provides a
complementary account of how perceptual information informs
behavior~\cite{fuster2004perception}. These accounts motivate our
distinction between understanding a social interaction and making a
judgment sensitive to the context within it; neither theory prescribes the
exact eight capabilities in PsycheMME.

Our taxonomy groups the eight capabilities into three domains.
\emph{Perceptually Grounded Mentalizing} distinguishes observable
interaction structure, interpretations of psychological states, and
support needs. \emph{Situated Empathic Responding} separates the timing,
verbal content, and physical or nonverbal form of a possible response.
\emph{Contextual and Normative Modulation} addresses relevant history
and social or safety constraints that may affect either understanding
or responding.

The domains provide diagnostic distinctions, not a compulsory
sequence from perception to action. In particular, Memory and Risk can shape
Timing, Verbal Response, or Action judgments without forming successive
reasoning stages. Nor does this taxonomy assert that the capabilities
are statistically independent psychological constructs: it specifies
which kind of judgment each benchmark question is designed to assess.

\subsubsection{Perceptually Grounded Mentalizing}

\paragraph{Social Grounding (G).}
Grounding identifies the participants, observable behavior, and
relations involved in an interaction. Questions may ask who speaks,
who is addressed, whose facial expression changes, what action occurs,
or how participants are positioned. Utterances, gaze, facial
expressions, gestures, and actions must be associated with the correct
people, using turn structure and spatial context when relevant.
Assigning an observable cue to its source establishes what was seen or
heard; interpreting the person's unobservable state belongs to W.

\paragraph{Psychological Understanding (W).}
Psychological Understanding concerns a person's state and its possible
causes or changes during the observed interaction. The model may need
to combine language, facial expression, behavior, and situational
context. These cues can be consistent, complementary, or conflicting:
for example, a reassuring utterance may coexist with hesitant
behavior. An interpretation should account for the available cues
rather than take any single cue as conclusive. The target is an
account of the interaction supported by observed cues, not a clinical
diagnosis or direct access to private mental experience. Latent
states remain inferences even when they are plausible.

\paragraph{Need Inference (N).}
Need Inference concerns the desired support or change and whether that
support is welcome. An explicit request may specify the need, whereas
hesitation, refusal, repeated difficulty, or emotional reactions may
require contextual interpretation. Recognizing difficulty is not the
same as knowing whether someone wants practical help, emotional
acknowledgment, clarification, or room to continue independently.
N therefore distinguishes a potentially useful intervention from a
wanted one. It does not decide when to intervene (T) or which response
or action should be chosen (S/A).

\subsubsection{Situated Empathic Responding}

\paragraph{Interaction Timing and Attunement (T).}
Timing evaluates whether a response or intervention is appropriate at
the observed moment. The alternatives may include speaking, waiting,
continuing to listen, or refraining from intervention. Relevant cues
include ongoing speech, pauses, turn-taking, activity demands,
urgency, and changes in the interaction. A pause does not always invite
an immediate reply, and a recognizable need does not automatically
justify interrupting. PsycheMME evaluates an offline judgment of
situational timing; it does not measure the latency or turn management
of a deployed streaming system.

\paragraph{Empathic Verbal Responding (S).}
Verbal Responding addresses what to say and how to say it, given the
person's state, need, and context. Appropriate content, strategy, and
tone may involve acknowledgment, validation, clarification, advice,
or restraint. A lengthy or warmly worded response is not necessarily
more appropriate than a brief one. The distinction from N is whether
a response is suitable, rather than which underlying support is wanted;
the distinction from T is the choice of words and strategy rather than
the moment to respond.

\paragraph{Embodied Social Action (A).}
Action concerns selecting a suitable physical or nonverbal behavior,
such as approaching or stepping back, offering assistance, handing
over an object, gesturing, or adjusting interpersonal distance. Such
choices depend on physical circumstances as well as the person's
expressed preferences and boundaries. Identifying an action that has
already occurred is a G judgment; selecting a suitable subsequent
behavior is an A judgment. The benchmark assesses the choice, not the
successful physical execution of a robotic action.

\subsubsection{Contextual and Normative Modulation}

\paragraph{Interaction and Profile Memory (M).}
Memory concerns using relevant available history to maintain
continuity in understanding and responding~\cite{nie2026personavlm}.
\emph{Interaction memory} includes earlier events, utterances,
requests, refusals, and interaction outcomes. \emph{Profile memory}
includes relatively stable, individual preferences, habits,
personal boundaries, and past choices. The distinction identifies
kinds of historical information used in a question; it does not imply
that the benchmark separately establishes memory competence for each
type. A preference or trait cannot be inferred as settled merely from
an isolated behavior in the current scene. The required history must
be available in the supplied context.

\paragraph{Risk, Boundary, and Autonomy Regulation (R).}
Risk concerns potential harm in interaction judgments, motivated by
embodied safety evaluation~\cite{ying2026agentsafe}.
PsycheMME additionally considers consent, boundaries, and autonomy.
A possible response
may be useful in principle yet inappropriate if it conflicts with an
expressed refusal or assumes permission to act. Risk may therefore
require revising, delaying, or withholding a response or action. A
person's need for assistance does not itself constitute consent to
receive it. R differs from N by assessing constraints on intervention,
not only the support the person may need.

\subsection{Capability Boundaries and Cue Constraints}
\label{app:capability_boundaries}

\paragraph{From observation to state, need, and timing.}
Consider a person attempting a task repeatedly, frowning, and asking
another participant to let them finish explaining. G concerns which
participant performs the task and speaks. W concerns what interpretation
of their state is supported by the behavior and words. N concerns what
kind of support, if any, they want. T concerns whether this moment
calls for intervention or continued listening. The same observations
can thus support distinct judgments without fixing all of their
answers in advance.

\paragraph{Observed actions versus response decisions.}
Suppose one participant holds an object toward another. Identifying who
holds or receives it targets G. Choosing a suitable acknowledgment or
clarification targets S. Deciding whether to accept it, assist with the
transfer, or step back targets A. The latter judgments may require
additional context about the exchange, including requests and refusals,
rather than recognition of the gesture alone.

\paragraph{Historical preferences and present constraints.}
Suppose the supplied history records a preference for verbal guidance
rather than physical assistance. Applying that preference targets M;
choosing appropriate verbal or physical assistance concerns S or A.
If the person now refuses help, R concerns respecting the present
boundary. Earlier preferences inform the interpretation but cannot
override current consent or refusal.

\paragraph{Limits of psychological interpretation.}
Observable expressions, utterances, and behavior can admit multiple
psychological explanations. PsycheMME does not require a unique
reconstruction of hidden states. Instead, an inference or proposed
interaction judgment should be supported by the available cues.
An interpretation is not justified simply because it is generally
plausible or does not contradict one isolated cue. Similarly, unknown
personal histories, preferences, or permissions should not be assumed.
This boundary on interpreting cues applies to both the reference QA construction
process and evaluation of rationales generated by models.

\subsection{Video Collection and Candidate Screening}
\label{app:video_curation_details}

Candidate material comes from Ego4D, EgoCom, MERCI+, CASTLE, EasyCom,
and IndEgo, supplemented by public first-person vlogs, interviews,
and recordings of daily life. These sources provide diverse social
settings rather than a single scripted interaction format. We select
clips for which a question about people, their interactions, or
responding appropriately to the context can be linked to cues present in the
recording.

Human screening assisted by VLMs first considers whether an episode
contains relevant social interaction and sufficiently clear behavioral
cues, such as speech, visible reactions, expressions, or gestures.
Visual quality screening excludes or trims distracting borders,
overlays, substantial occlusion, and extended transitions when they
obscure relevant cues. Psychology Knowledge guides construct relevance
checks during question construction. The selection criterion is not simply that a scene
appears emotional or socially interesting: the eventual question must
be answerable from the available video and public context, without
requiring access to a participant's unobserved private state.

\subsection{QA Construction with Independent Answering}
\label{app:construction_details}

The question construction framework in Fig.~\ref{fig:construction} generates questions, reasons independently, critiques outputs, and
refines candidates. Its main design
choice is to separate the answer proposed when a question is written
from an independent attempt to answer that question. This separation
reduces the risk that a generated reference is accepted only because
the same agent can justify its own proposal.

\paragraph{Question proposal.}
The Question Agent receives the source clip, available public
context, and a target capability. It proposes a question, answer,
options when applicable, and supporting cues. The proposed answer,
cues supporting the proposal, and private rationale remain in a restricted
state. This proposal is a candidate for verification, not accepted
reference truth.

\paragraph{Independent reasoning and information isolation.}
The Answer Agent examines the video again with only the
question, available answer options, and public context. It cannot see
the proposed answer, cues supporting the proposal, or private rationale.
Before producing an independent answer and supporting rationale, it
checks whether the question is answerable from the available cues. It
may flag ambiguity or insufficient support instead of forcing an
answer. Agreement between the two paths is therefore more informative
than simply asking the Question Agent to reconsider its own output,
but agreement alone does not establish correctness.

\paragraph{Critique and refinement.}
The Critic Agent compares the independent reasoning path and the
proposal against the observed cues. Its checks concern
answerability, cue support, logical coherence, and construct
alignment. Questions with defects in the proposal return to the
Question Agent; problems in the reasoning path trigger another examination by the
Answer Agent. Psychology Knowledge guides all three agents' construct
alignment and psychological interpretation grounded in observed cues.
Candidates are revised or rejected for construct mismatches or
unsupported attributions and discarded if they still fail verification
after at most two refinement rounds.

\paragraph{Shared state and access rules.}
The construction framework uses a Shared State to record verification feedback,
refinement history, and capability coverage. Access based on agent roles
separates information needed for independent answering from private
proposal information. The state can also guide further question
proposal toward capabilities that remain underrepresented. This is a
mechanism for quality control and coverage; it does not establish
that every proposed item is correct before human review.

\subsection{Human Quality Verification and Data Separation}
\label{app:quality_details}

Using Qwen3.5-27B and Qwen3.5-397B-A17B, the construction framework produces more
than 10,000 candidate QA pairs. Five researchers with psychology
backgrounds independently review the candidates. Their review addresses whether the question is
valid and answerable, whether the proposed answer is correct, and
whether the psychological interpretation is consistent with the
observed cues. Only unanimously approved items are retained as
benchmark questions.

Material for instruction tuning is filtered separately and kept disjoint
from the benchmark split. Its selection and use in further training are
covered in Appendix~\ref{app:post_training_details}. These quality
checks complement, rather than replace, the independent generation and
critique stages: machine verification helps identify candidates,
while human review determines whether an item enters the released
benchmark.

\subsection{Benchmark Composition and Question Formats}
\label{app:composition_details}

The benchmark contains 630 video episodes recorded in real settings and 1,000
questions. There are 890 choice questions and 110 open questions. Questions are categorized by
the principal capability being assessed, with counts of 186 (G), 320
(W), 97 (N), 72 (T), 97 (S), 94 (A), 61 (M), and 73 (R).
This distribution is not uniform: in particular, W contributes many
more items than T or M. Consequently, the principal reported score is
an unweighted macro average across the eight capabilities rather than
an overall micro average across questions. Figure~\ref{fig:benchmark_statistics}
visualizes the finer taxonomy, source and structure of question formats,
and video and distributions of question lengths.


\subsection{Detailed Answer and Rationale Evaluation}
\label{app:scoring_details}

\paragraph{Answer Correctness.}
The normalized answer score $a_i\in[0,1]$ is evaluated
independently of the rationale. Choice answers use Exact Match for
one required option and Exact-set Match for a complete option set.
Open answers are evaluated by a
fixed semantic judge against references reviewed by humans
and known facts, allowing equivalent interpretations.
Open-ended scores take values $0$, $0.5$, or $1$.

\paragraph{Rationale Presence.}
The binary indicator $c_i\in\{0,1\}$ records whether an
explicit rationale is provided. It does not require all
eight rationale fields to be populated, as some fields
may be irrelevant to a given question. Missing or
unevaluable rationales receive zero verified credit.

\paragraph{Evidence Support and Logical Integrity.}
A fixed judge evaluates rationales against frozen cue annotations.
Evidence Support assesses whether claims are supported
by observable cues without unsupported psychological
attribution. Logical Integrity checks consistency across
rationale fields and with the final answer.

Both dimensions use four levels with multipliers
$1.2$, $1.0$, $0.8$, and $0.5$.
For Evidence Support, these correspond to
\emph{strong}, \emph{normal}, \emph{weak}, and
\emph{contradicted}; for Logical Integrity, they
correspond to \emph{fully coherent}, \emph{acceptable},
\emph{weak}, and \emph{contradictory}.
Insufficient support or unevaluable judgments receive
zero verified credit. Supported alternative interpretations
are allowed, but the absence of contradiction alone does not
establish sufficient support from observed cues.

\paragraph{Score Aggregation.}
Let $e_i$ and $\ell_i$ denote the Evidence Support and Logical Integrity
multipliers. The normalization factor $\lambda^2$, with $\lambda=1.2$, in
Eq.~\ref{eq:psychebench_score} normalizes the maximum
verified credit to $1$.

The overall Reasoning-Verified score is
\begin{equation}
    S_{\mathrm{Psyche}} =
    \frac{100}{8}\sum_{c\in\mathcal C}
    \frac{1}{|\mathcal D_c|}
    \sum_{i\in\mathcal D_c}s_i,
    \label{eq:app_macro_score}
\end{equation}
where $\mathcal C$ contains the eight capabilities and
$\mathcal D_c$ denotes the questions in capability $c$.
Raw Answer uses the same macro average with $a_i$
instead of $s_i$.

\paragraph{Score Interpretation.}
A correct answer with normal Evidence Support and
acceptable logic receives $1/\lambda^2\approx69.44\%$
verified credit, even with an explicit rationale.
Consequently, the gap between Raw and Verified scores includes rubric
weighting and should not be interpreted as a direct
rate of reasoning errors. The metric evaluates explicit
rationales rather than unobserved internal reasoning.
