# Supplementary material for: PsycheMME: A Psychology-Informed Benchmark for Social Understanding and Interaction in Videos
Source: arXiv:2610.28625 source file (2026-10-20)
Supplement: Supplementary file 3 [file understanding_interaction.tex]

\section{Exploratory Analysis of Understanding and Decisions}
\label{app:understanding_interaction}

\subsection{Linked Question Pairs for Qwen}
\label{app:linked_pairs}

For Qwen3.5-9B, we examine the association between understanding
and decision correctness on 173 links from 101 episodes:
57 Timing, 69 Verbal Response, and 47 Action links.
The links contain 148 unique understanding questions and 116 unique
decision questions. A question can occur in several links;
confidence intervals therefore resample episodes.

Decision accuracy is 60.13\% when the linked understanding answer
is correct and 26.67\% when it is incorrect, a difference of
33.46 points (95\% CI $[5.80,56.25]$;
Table~\ref{tab:app_ud}). This exploratory result describes an
association for Qwen on this subset; it does not establish a causal
dependence or a pattern across models.
\input{table/understanding_decisions}
